# Supplementary material for: Structured penalized regression for drug sensitivity prediction
Source: arXiv:1902.04996 source file (2020-03-08)
Supplement: Supplementary file 1 [file Manuscript_Suppl.pdf]

# SUPPLEMENTARY MATERIALS FOR "STRUCTURED PENALIZED REGRESSION FOR DRUG SENSITIVITY PREDICTION"

By Zhi Zhao and Manuela Zucknick

*Department of Biostatistics, University of Oslo*
*P.O.Box 1122 Blindern 0317 Oslo, Norway*

## S1. Theorem 1.

Theorem 1. *Given $n$ samples and $m$ responses $\mathbf{Y}$, standardized $S$ data sources $\mathbf{X} = [\mathbf{X}_1, \cdots, \mathbf{X}_S]$ (variance 1 and mean 0 for each column) with numbers of features $p_1, \cdots, p_S$, respectively, and the corresponding coefficients matrix $\mathbf{B}$, let $\boldsymbol{\lambda} = (\lambda_1, \cdots, \lambda_S)$, and $\hat{\boldsymbol{\beta}}_0(\boldsymbol{\lambda}, \alpha)$, $\hat{\mathbf{B}}(\boldsymbol{\lambda}, \alpha)$ be the sIPF-elastic-net estimates. Suppose two coefficients $\beta_{jk}$ and $\beta_{j'k}$ from the sth and $s'$th data sources ($j, j' \in [p], j \neq j'; s, s' \in [S]; k \in [m]$), respectively, and $\hat{\beta}_{jk}(\boldsymbol{\lambda}, \alpha)\hat{\beta}_{j'k}(\boldsymbol{\lambda}, \alpha) > 0$; then*

$$|\hat{\beta}_{jk}(\boldsymbol{\lambda}, \alpha) - \hat{\beta}_{j'k}(\boldsymbol{\lambda}, \alpha)| \leq \frac{\sqrt{\lambda_s^2 + \lambda_{s'}^2 - 2\lambda_s\lambda_{s'}\rho}}{mn\lambda_s\lambda_{s'}(1-\alpha)}\|\mathbf{Y}\|_{\ell_1},$$

*where sample correlation $\rho = \boldsymbol{x}_{s,j}^\top \boldsymbol{x}_{s',j'}$ with $\boldsymbol{x}_{s,j}$ the vector of $n$ samples of the $j$th feature belonging to the sth data source and $\|\mathbf{Y}\|_{\ell_1} = \sum_{i=1}^n \sum_{k=1}^m |y_{ik}|$.*

Proof. Let

$$\mathcal{L}(\boldsymbol{\lambda}, \alpha, \boldsymbol{\beta}_0, \mathbf{B}) = \frac{1}{2mn}\|\mathbf{Y} - \mathbf{1}_n\boldsymbol{\beta}_0^\top - \mathbf{X}\mathbf{B}\|_F^2 + \sum_{s=1}^S \lambda_s(\alpha\|\mathbf{B}\|_{\ell_1} + \frac{1}{2}(1-\alpha)\|\mathbf{B}\|_{\ell_2}^2).$$

If $\hat{\beta}_{jk}(\boldsymbol{\lambda}, \alpha)\hat{\beta}_{j'k}(\boldsymbol{\lambda}, \alpha) > 0$, then both $\hat{\beta}_{jk}(\boldsymbol{\lambda}, \alpha)$ and $\hat{\beta}_{j'k}(\boldsymbol{\lambda}, \alpha)$ are nonzero, and we have $\mathrm{sgn}\{\hat{\beta}_{j'k}(\boldsymbol{\lambda}, \alpha)\} = \mathrm{sgn}\{\hat{\beta}_{j'k}(\boldsymbol{\lambda}, \alpha)\}$. Because of the solution

$$(\hat{\boldsymbol{\beta}}_0(\boldsymbol{\lambda}, \alpha), \hat{\mathbf{B}}(\boldsymbol{\lambda}, \alpha)) = \arg\min_{\boldsymbol{\beta}_0, \mathbf{B}} \left\{ \frac{1}{2mn}\|\mathbf{Y} - \mathbf{1}_n\boldsymbol{\beta}_0^\top - \mathbf{X}\mathbf{B}\|_F^2 + \sum_{s=1}^S \lambda_s(\alpha\|\mathbf{B}_s\|_{\ell_1} + \frac{1}{2}(1-\alpha)\|\mathbf{B}_s\|_{\ell_2}^2) \right\},$$

if $\hat{\beta}_{jk} \neq 0$, $\hat{\boldsymbol{\beta}}_0(\boldsymbol{\lambda}, \alpha)$ and $\hat{\mathbf{B}}(\boldsymbol{\lambda}, \alpha)$ satisfy

$$\left.\frac{\partial \mathcal{L}(\boldsymbol{\lambda}, \alpha, \boldsymbol{\beta}_0, \mathbf{B})}{\partial \beta_{jk}}\right|_{\substack{\boldsymbol{\beta}_0 = \hat{\boldsymbol{\beta}}_0(\boldsymbol{\lambda}, \alpha) \\ \mathbf{B} = \hat{\mathbf{B}}(\boldsymbol{\lambda}, \alpha)}} = 0.$$

Then we have

$$-\frac{1}{mn}\boldsymbol{x}_{s,j}^\top\{\boldsymbol{y}_k - \mathbf{X}\hat{\boldsymbol{\beta}}_k(\boldsymbol{\lambda}, \alpha)\} + \lambda_s\left[\alpha\ \mathrm{sgn}\{\hat{\beta}_{jk}(\boldsymbol{\lambda}, \alpha)\} + (1-\alpha)\hat{\beta}_{jk}(\boldsymbol{\lambda}, \alpha)\right] = 0,$$
$$-\frac{1}{mn}\boldsymbol{x}_{s',j'}^\top\{\boldsymbol{y}_k - \mathbf{X}\hat{\boldsymbol{\beta}}_k(\boldsymbol{\lambda}, \alpha)\} + \lambda_{s'}\left[\alpha\ \mathrm{sgn}\{\hat{\beta}_{j'k}(\boldsymbol{\lambda}, \alpha)\} + (1-\alpha)\hat{\beta}_{j'k}(\boldsymbol{\lambda}, \alpha)\right] = 0,$$

where $\hat{\boldsymbol{\beta}}_k(\boldsymbol{\lambda}, \alpha)$ is the $k$th column of $\hat{\boldsymbol{B}}(\lambda, \alpha)$. Hence we have

$$\frac{1}{mn}(\lambda_{s'}\boldsymbol{x}_{s',j'}^\top - \lambda_s \boldsymbol{x}_{s,j}^\top)\{\boldsymbol{y}_k - \mathbf{X}\hat{\boldsymbol{\beta}}_k(\boldsymbol{\lambda}, \alpha)\} + \lambda_s\lambda_{s'}(1-\alpha)\{\hat{\beta}_{jk}(\boldsymbol{\lambda}, \alpha) - \hat{\beta}_{j'k}(\boldsymbol{\lambda}, \alpha)\} = 0.$$

Let $\hat{r}(\boldsymbol{\lambda}, \alpha) = y_k - \mathbf{X}\hat{\boldsymbol{\beta}}_k(\boldsymbol{\lambda}, \alpha)$. Then

$$\frac{1}{2mn}\|\hat{r}(\boldsymbol{\lambda}, \alpha)\|_2^2 \le \mathcal{L}\{\boldsymbol{\lambda}, \alpha, \hat{\boldsymbol{\beta}}_0(\boldsymbol{\lambda}, \alpha), \hat{\mathbf{B}}(\boldsymbol{\lambda}, \alpha)\} \le \mathcal{L}\{\boldsymbol{\lambda}, \alpha, \boldsymbol{\beta}_0 = 0, \mathbf{B} = 0\} = \frac{1}{2mn}\|\mathbf{Y}\|_F^2.$$

So $|\hat{r}(\boldsymbol{\lambda}, \alpha)| \le \|\mathbf{Y}\|_{\ell_1}$. Since $\mathbf{X}$ is standardized, i.e., $\|\boldsymbol{x}_{s,j}\|_2^2 = 1$ and $\|\boldsymbol{x}_{s,j}\|_1 = 0$, then $\|\lambda_s \boldsymbol{x}_{s,j}^\top - \lambda_{s'}\boldsymbol{x}_{s',j'}^\top\|_2^2 = \lambda_s^2 + \lambda_{s'}^2 - 2\lambda_s\lambda_{s'}\rho$ where $\rho = \boldsymbol{x}_{s,j}^\top \boldsymbol{x}_{s',j'}$. Therefore,

$$\begin{aligned}
|\hat{\beta}_{jk}(\boldsymbol{\lambda}, \alpha) - \hat{\beta}_{j'k}(\boldsymbol{\lambda}, \alpha)| &\le \frac{1}{mn\lambda_s\lambda_{s'}(1-\alpha)}\|(\lambda_s \boldsymbol{x}_{s,j}^\top - \lambda_{s'}\boldsymbol{x}_{s',j'}^\top\|_2 |\hat{r}(\boldsymbol{\lambda}, \alpha)| \\
&\le \frac{\sqrt{\lambda_s^2 + \lambda_{s'}^2 - 2\lambda_s\lambda_{s'}\rho}}{mn\lambda_s\lambda_{s'}(1-\alpha)}\|\mathbf{Y}\|_{\ell_1}.
\end{aligned}$$

□

## S2. A Proposition of IPF-tree-lasso.

PROPOSITION. *Given response* $\mathbf{Y}$ *and* $S$ *data sources* $\mathbf{X} = [\mathbf{X}_1, \dots, \mathbf{X}_S]$ *with numbers of features* $p_1, \dots, p_S$*, respectively, and the corresponding coefficients matrix is* $\mathbf{B} = [\mathbf{B}_1 \vdots \cdots \vdots \mathbf{B}_S]$*, let*

$$\mathbf{X}^\star = \left[\mathbf{X}_1, \tfrac{\lambda_1}{\lambda_2}\mathbf{X}_2, \cdots, \tfrac{\lambda_1}{\lambda_S}\mathbf{X}_S\right] \in \mathbb{R}^{n \times (p_1 + \cdots + p_S)},$$

$$\mathbf{B}^\star = \left[\mathbf{B}_1 \vdots \tfrac{\lambda_2}{\lambda_1}\mathbf{B}_2 \vdots \cdots \vdots \tfrac{\lambda_S}{\lambda_1}\mathbf{B}_S\right] \in \mathbb{R}^{(p_1 + \cdots + p_S) \times n},$$

$$(\hat{\boldsymbol{\beta}}_0, \hat{\mathbf{B}}) = \underset{\boldsymbol{\beta}_0, \mathbf{B}}{\arg\min}\left\{\frac{1}{2mn}\|\mathbf{Y} - \mathbf{1}_n\boldsymbol{\beta}_0^\top - \mathbf{X}\mathbf{B}\|_F^2 + \sum_{s=1}^S \lambda_s \left(\sum_{j=1}^{p_s}\sum_{\nu \in V_{int}} \omega_\nu \|\boldsymbol{\beta}_{j,s}^{G_\nu}\|_{\ell_2} + \sum_{j=1}^{p_s}\sum_{\nu \in V_{leaf}} \|\boldsymbol{\beta}_{j,s}^{G_\nu}\|_{\ell_2}\right)\right\},$$

$$(\hat{\boldsymbol{\beta}}_0, \hat{\mathbf{B}}^\star) = \underset{\boldsymbol{\beta}_0, \mathbf{B}^\star}{\arg\min}\left\{\frac{1}{2mn}\|\mathbf{Y} - \mathbf{1}_n\boldsymbol{\beta}_0^\top - \mathbf{X}^\star\mathbf{B}^\star\|_F^2 + \lambda_1 \left(\sum_{j}^{p}\sum_{\nu \in V_{int}} \omega_\nu \|\boldsymbol{\beta}_{j}^{\star G_\nu}\|_{\ell_2} + \sum_{j}^{p}\sum_{\nu \in V_{leaf}} \|\boldsymbol{\beta}_{j}^{\star G_\nu}\|_{\ell_2}\right)\right\}.$$

*Then* $\hat{\mathbf{B}}^\star = \left[\hat{\mathbf{B}}_1 \vdots \tfrac{\lambda_2}{\lambda_1}\hat{\mathbf{B}}_2 \vdots \cdots \vdots \tfrac{\lambda_S}{\lambda_1}\hat{\mathbf{B}}_S\right]$*, where* $\hat{\mathbf{B}} = [\hat{\mathbf{B}}_1 \vdots \hat{\mathbf{B}}_2 \vdots \cdots \vdots \hat{\mathbf{B}}_S]$.

PROOF. W.L.O.G., we here give the proof in the case with three responses and a tree of five nodes that consists of three leaf nodes, one internal node (not root node) and one root node, illustrated in Figure 2, and two data sources.

Let leaf nodes $V_{\text{leaf}} = \{\nu_1, \nu_2, \nu_3\}$, internal nodes $V_{\text{int}} = \{\nu_4, \nu_5\}$, and the transformation

$$\mathbf{X}^\star = [\mathbf{X}_1, \frac{\lambda_1}{\lambda_2}\mathbf{X}_2],$$

$$\mathbf{B}\star = \begin{bmatrix} \mathbb{I}_{p_1} & 0 \\ 0 & \frac{\lambda_2}{\lambda_1}\mathbb{I}_{p_2} \end{bmatrix} \mathbf{B}.$$

Let

$$\begin{aligned}
&\|\boldsymbol{\beta}_j^{\star G_{\nu_1}}\|_{\ell_2} = |\beta_{j1}^\star|, \quad \|\boldsymbol{\beta}_j^{\star G_{\nu_3}}\|_{\ell_2} = |\beta_{j2}^\star|, \quad \|\boldsymbol{\beta}_j^{\star G_{\nu_3}}\|_{\ell_2} = |\beta_{j3}^\star|, \\
&\|\boldsymbol{\beta}_j^{\star G_{\nu_4}}\|_{\ell_2} = \sqrt{(\beta_{j1}^\star)^2 + (\beta_{j2}^\star)^2}, \\
&\|\boldsymbol{\beta}_j^{\star G_{\nu_5}}\|_{\ell_2} = \sqrt{(\beta_{j1}^\star)^2 + (\beta_{j2}^\star)^2 + (\beta_{j3}^\star)^2}.
\end{aligned}$$

Then the new objective function is

$$\begin{aligned}
&\min_{\boldsymbol{\beta}_0, \mathbf{B}^\star} \frac{1}{2}\|\mathbf{Y} - \mathbf{1}_n\boldsymbol{\beta}_0^\top - \mathbf{X}^\star\mathbf{B}^\star\|_F^2 + \lambda_1 \sum_j \sum_{\nu\in V_{\text{int}}} \omega_\nu \|\boldsymbol{\beta}_j^{\star G_\nu}\|_{\ell_2} + \lambda_1 \sum_j \sum_{\nu\in V_{\text{leaf}}} \omega_\nu \|\boldsymbol{\beta}_j^{\star G_\nu}\|_{\ell_2} \\
&= \min_{\boldsymbol{\beta}_0, \mathbf{B}^\star} \frac{1}{2}\|\mathbf{Y} - \mathbf{1}_n\boldsymbol{\beta}_0^\top - \mathbf{X}^\star\mathbf{B}^\star\|_F^2 + \lambda_1 \sum_{j,k} \omega_{\nu_k} |\beta_{jk}^\star| \\
&+ \lambda_1 \sum_j \{g_{\nu_4} \|\boldsymbol{\beta}_j^{\star G_{\nu_4}}\|_{\ell_2} + s_{\nu_4}(\beta_{j1}^\star + (\beta_{j2}^\star)\} \\
&+ \lambda_1 \sum_j \{g_{\nu_5} \|\boldsymbol{\beta}_j^{\star G_{\nu_5}}\|_{\ell_2} + s_{\nu_5} g_{\nu_4} \|\boldsymbol{\beta}_j^{\star G_{\nu_4}}\|_{\ell_2} + s_{\nu_5} s_{\nu_4}(\beta_{j1}^\star + (\beta_{j2}^\star) + s_{\nu_5}\beta_{j3}^\star\} \\
&= \min_{\boldsymbol{\beta}_0, \mathbf{B}} \frac{1}{2}\left\|\mathbf{Y} - \left[\mathbf{X}_1, \frac{\lambda_1}{\lambda_2}\mathbf{X}_2\right] \begin{bmatrix} \mathbb{I}_{p_1} & 0 \\ 0 & \frac{\lambda_2}{\lambda_1}\mathbb{I}_{p_2} \end{bmatrix} \mathbf{B} \right\|_F^2 + \lambda_1 \sum_{j=1}^{p_1} \sum_{k=1}^{m} \omega_{\nu_k} |\beta_{jk}| + \lambda_2 \sum_{j=p_1+1}^{p_1+p_2} \sum_{k=1}^{m} \omega_{\nu_k} |\beta_{jk}| \\
&+ \lambda_1 \sum_{j=1}^{p_1} \{g_{\nu_4} \|\boldsymbol{\beta}_j^{G_{\nu_4}}\|_{\ell_2} + s_{\nu_4}(\beta_{j1} + (\beta_{j2})] + \lambda_2 \sum_{j=p_1+1}^{p_1+p_2} [g_{\nu_4} \|\boldsymbol{\beta}_j^{G_{\nu_4}}\|_{\ell_2} + s_{\nu_4}(\beta_{j1} + (\beta_{j2})\} \\
&+ \lambda_1 \sum_{j=1}^{p_1} \{g_{\nu_5} \|\boldsymbol{\beta}_j^{G_{\nu_5}}\|_{\ell_2} + s_{\nu_5} g_{\nu_4} \|\boldsymbol{\beta}_j^{G_{\nu_4}}\|_{\ell_2} + s_{\nu_5} s_{\nu_4}(\beta_{j1} + (\beta_{j2}) + s_{\nu_5}\beta_{j3}\} \\
&+ \lambda_2 \sum_{j=p_1+1}^{p_1+p_2} \{g_{\nu_5} \|\boldsymbol{\beta}_j^{G_{\nu_5}}\|_{\ell_2} + s_{\nu_5} g_{\nu_4} \|\boldsymbol{\beta}_j^{G_{\nu_4}}\|_{\ell_2} + s_{\nu_5} s_{\nu_4}(\beta_{j1} + (\beta_{j2}) + s_{\nu_5}\beta_{j3}\} \\
&= \min_{\boldsymbol{\beta}_0, \mathbf{B}} \frac{1}{2}\|\mathbf{Y} - \mathbf{1}_n\boldsymbol{\beta}_0^\top - \mathbf{X}\mathbf{B}\|_F^2 + \lambda_1 \sum_{j=1}^{p_1} \left( \sum_{\nu\in V_{\text{int}}} \omega_\nu \|\boldsymbol{\beta}_j^{G_\nu}\|_{\ell_2} + \sum_{\nu\in V_{\text{leaf}}} \omega_\nu \|\boldsymbol{\beta}_j^{G_\nu}\|_{\ell_2} \right) \\
&+ \lambda_2 \sum_{j=p_1+1}^{p_1+p_2} \left( \sum_{\nu\in V_{\text{int}}} \omega_\nu \|\boldsymbol{\beta}_j^{G_\nu}\|_{\ell_2} + \sum_{\nu\in V_{\text{leaf}}} \omega_\nu \|\boldsymbol{\beta}_j^{G_\nu}\|_{\ell_2} \right).
\end{aligned}$$

□

**S3. Directly adapting the algorithm of tree-lasso to IPF-tree-lasso.**

**S3.1 Directly adapted IPF-tree-lasso without non-penalized features**

Compared to the independent responses in elastic-net and IPF-lasso, Kim and Xing [1] proposed tree-lasso to consider the hierarchical structure over the multivariate (even high

dimensional) responses. The response variables can be represented as tree $T$ with a set of vertices $V$ and groups $G_\nu$ which is given based on external information or data driven like hierarchical clustering algorithm used in the paper. Considering response $\mathbf{Y} \in \mathbb{R}^{n\times m}$ and two data sources $\mathbf{X} = [\mathbf{X}_1, \mathbf{X}_2] \in \mathbb{R}^{n\times(p_1+p_2)}$, let $\mathbf{B} = [\mathbf{B}_1\vdots\mathbf{B}_2] \in \mathbb{R}^{(p_1+p_2)\times m}$ and $\mathbf{B}_s$ $(s = 1, 2)$ is the coefficients matrix corresponding to the $s$th data source. The tree lasso is defined as

$$\min_{\boldsymbol{\beta}_0,\mathbf{B}_1,\mathbf{B}_2} \frac{1}{2}\|\mathbf{Y} - \mathbf{1}\beta_0^\top - \mathbf{X}_1\mathbf{B}_1 - \mathbf{X}_2\mathbf{B}_2\|_F^2 + \lambda\sum_j \sum_{\nu\in V_{\text{int}}} \omega_\nu \|\boldsymbol{\beta}_j^{G_\nu}\|_{\ell_2} + \lambda\sum_j \sum_{\nu\in V_{\text{leaf}}} \omega_\nu \|\boldsymbol{\beta}_j^{G_\nu}\|_{\ell_2},$$

where $\boldsymbol{\beta}_j^{G_\nu} = \{\beta_{jk} : k \in G_\nu\}$ is the $j$th row of $\mathbf{B}$ associated with $k$th response, and $\omega_\nu$ is the group weight either associated with height of each internal node or $\omega_\nu = 1$ corresponding a leaf node. Here, for the convenience, we use factor $\frac{1}{2}$ before the loss function.

Then the penalty term involving internal nodes is

$$\begin{aligned}
\Omega(\mathbf{B}_1, \mathbf{B}_2) &= \lambda_1 \sum_{j=1}^{p_1} \sum_{\nu\in V_{\text{int}}} \omega_\nu \|\boldsymbol{\beta}_j^{G_\nu}\|_{\ell_2} + \lambda_2 \sum_{j=p_1+1}^{p_1+p_2} \sum_{\nu\in V_{\text{int}}} \omega_\nu \|\boldsymbol{\beta}_j^{G_\nu}\|_{\ell_2} \\
&= \lambda_1 \sum_{j=1}^{p_1} \sum_{\nu\in V_{\text{int}}} \omega_\nu \max_{\|\boldsymbol{\alpha}_j^{G_\nu}\|_{\ell_2}\le 1} (\boldsymbol{\alpha}_j^{G_\nu})^\top \boldsymbol{\beta}_j^{G_\nu} + \lambda_2 \sum_{j=p_1+1}^{p_1+p_2} \sum_{\nu\in V_{\text{int}}} \omega_\nu \max_{\|\boldsymbol{\alpha}_j^{G_\nu}\|_{\ell_2}\le 1} (\boldsymbol{\alpha}_j^{G_\nu})^\top \boldsymbol{\beta}_j^{G_\nu} \\
&= \max_{\mathbf{A}_1\in\mathcal{Q}_1} \langle C_1\mathbf{B}_1^\top, \mathbf{A}_1\rangle + \max_{\mathbf{A}_2\in\mathcal{Q}_2} \langle C_2\mathbf{B}_2^\top, \mathbf{A}_2\rangle,
\end{aligned}$$

where $\mathcal{Q}_1 = \{\mathbf{A}_1 : \|\boldsymbol{\alpha}_j^{G_\nu}\|_{\ell_2} \le 1, \forall j \in \{1, \dots, p_1\}, \nu \in V_{\text{int}}\}$, $\mathcal{Q}_1 = \{\mathbf{A}_2 : \|\boldsymbol{\alpha}_j^{G_\nu}\|_{\ell_2} \le 1, \forall j \in \{p_1 + 1, \dots, p_1 + p_2\}, \nu \in V_{\text{int}}\}$, $C_1 = \lambda_1 C$, $C_2 = \lambda_2 C$ and

$$C^k_{(\nu,i)} = \begin{cases} \omega_\nu & \text{if } k \in G_\nu \\ 0 & \text{otherwise} \end{cases}, \mathbf{A}_1 = \begin{bmatrix} \boldsymbol{\alpha}_1^{G_1} & \dots & \boldsymbol{\alpha}_{p_1}^{G_1} \\ \vdots & \ddots & \vdots \\ \boldsymbol{\alpha}_1^{G_{|V_{\text{int}}|}} & \dots & \boldsymbol{\alpha}_{p_1}^{G_{|V_{\text{int}}|}} \end{bmatrix}, \mathbf{A}_2 = \begin{bmatrix} \boldsymbol{\alpha}_{p_1+1}^{G_1} & \dots & \boldsymbol{\alpha}_{p_1+p_2}^{G_1} \\ \vdots & \ddots & \vdots \\ \boldsymbol{\alpha}_{p_1+1}^{G_{|V_{\text{int}}|}} & \dots & \boldsymbol{\alpha}_{p_1+p_2}^{G_{|V_{\text{int}}|}} \end{bmatrix}.$$

The smooth approximation to the nonsmooth penalty is

$$f_\mu(\mathbf{B}_1) + f_\mu(\mathbf{B}_2) = \max_{\mathbf{A}_1\in\mathcal{Q}_1} \langle C_1\mathbf{B}_1^\top, \mathbf{A}_1\rangle - \mu d(\mathbf{A}_1) + \max_{\mathbf{A}_2\in\mathcal{Q}_2} \langle C_2\mathbf{B}_2^\top, \mathbf{A}_2\rangle - \mu d(\mathbf{A}_2),$$

and the gradients are

$$\begin{aligned}
\nabla f_\mu(\mathbf{B}_1) &= (\mathbf{A}_1^*)^\top C_1, \\
\nabla f_\mu(\mathbf{B}_2) &= (\mathbf{A}_2^*)^\top C_2,
\end{aligned}$$

where $\mathbf{A}_s^* = (\boldsymbol{\alpha}_{j,s}^{G_\nu})* = S(\frac{\lambda\omega_\nu\boldsymbol{\beta}_{j,s}^{G_\nu}}{\mu})$, $s = 1, 2$, and $S(\cdot)$ is the shrinkage operator. Then we obtain the objective function

$$\begin{aligned}
\hat{\mathbf{B}}_T = \arg\min_{\beta_\mathbf{0},\mathbf{B}} \{ & \frac{1}{2}\|\mathbf{Y} - \mathbf{1}\beta_0^\top - \mathbf{X}_1\mathbf{B}_1 - \mathbf{X}_2\mathbf{B}_2\|_F^2 + f_\mu(\mathbf{B}_1) + f_\mu(\mathbf{B}_2) \\
& + \lambda_1 \sum_{j=1}^{p_1}\sum_{k=1}^{m} \omega_k|\beta_{jk}| + \lambda_2 \sum_{j=p_1+1}^{p_1+p_2}\sum_{k=1}^{m} \omega_k|\beta_{jk}| \},
\end{aligned}$$

where $\mathbf{B} = [\beta_0^\top \vdots \mathbf{B}_1 \vdots \mathbf{B}_2]$. The smooth part is

$$h(\mathbf{B}) = \frac{1}{2}\|\mathbf{Y} - \mathbf{1}\beta_0^\top - \mathbf{X}_1\mathbf{B}_1 - \mathbf{X}_2\mathbf{B}_2\|_F^2 + f_\mu(\mathbf{B}_1) + f_\mu(\mathbf{B}_2)$$

and its gradient is

$$\begin{aligned}\nabla h(\mathbf{B}) &= \begin{bmatrix}\nabla h(\beta_0^\top)\\ \nabla h(\mathbf{B}_1)\\ \nabla h(\mathbf{B}_2)\end{bmatrix}\\ &= \begin{bmatrix}\mathbf{1}^\top(\mathbf{1}\beta_0^\top + \mathbf{X}_1\mathbf{B}_1 + \mathbf{X}_2\mathbf{B}_2 - \mathbf{Y})\\ \mathbf{X}_1^\top(\mathbf{1}\beta_0^\top + \mathbf{X}_1\mathbf{B}_1 + \mathbf{X}_2\mathbf{B}_2 - \mathbf{Y}) + (\mathbf{A}_1^*)^\top C_1\\ \mathbf{X}_2^\top(\mathbf{1}\beta_0^\top + \mathbf{X}_1\mathbf{B}_1 + \mathbf{X}_2\mathbf{B}_2 - \mathbf{Y}) + (\mathbf{A}_2^*)^\top C_2\end{bmatrix}\\ &= \mathbf{X}^\top\mathbf{X}\begin{bmatrix}\beta_0^\top\\ \mathbf{B}_1\\ \mathbf{B}_2\end{bmatrix} - \mathbf{X}^\top\mathbf{Y} + \begin{bmatrix}0 & 0 & 0\\ 0 & (\mathbf{A}_1^*)^\top & 0\\ 0 & 0 & (\mathbf{A}_2^*)^\top\end{bmatrix}\begin{bmatrix}0\\ \lambda_1\mathbb{I}_{p_1}\\ \lambda_2\mathbb{I}_{p_2}\end{bmatrix}C,\end{aligned}$$

where $\mathbf{X} = [\mathbf{1}\ \mathbf{X}_1\ \mathbf{X}_2]$, and the corresponding Lipschitz constant

$$L = \lambda_{\max}(\mathbf{X}^\top\mathbf{X}) + \frac{1}{\mu}\left\|\begin{bmatrix}0\\ \lambda_1\mathbb{I}_{p_1}\\ \lambda_2\mathbb{I}_{p_2}\end{bmatrix}C\right\|^2.$$

Let $\mathbf{B} = \mathbf{W}^{(t)} - \frac{1}{L}\nabla h(\mathbf{W}^{(t)})$, by second Taylor approximation,

$$h(\mathbf{B}) \approx h(\mathbf{W}_t) + \langle \mathbf{B} - \mathbf{W}^{(t)}, \nabla h(\mathbf{W}^{(t)})\rangle + \frac{L}{2}\|\mathbf{B} - \mathbf{W}^{(t)}\|_{\ell_2}^2.$$

According to the proximal gradient method and ignoring the constant term,

$$\begin{aligned}\mathbf{B}^{(t+1)} &= \arg\min_{\mathbf{B}} Q_L(\mathbf{B}, \mathbf{W}^{(t)})\\ &= \arg\min_{\mathbf{B}}\left\{h(\mathbf{B}) + \boldsymbol{\omega}\left\|\begin{bmatrix}\lambda_1\mathbf{B}_1\\ \lambda_2\mathbf{B}_2\end{bmatrix}\right\|_{\ell_1}\right\}\\ &\approx \arg\min_{\mathbf{B}}\left\{h(\mathbf{W}^{(t)}) + \langle \mathbf{B} - \mathbf{W}^{(t)}, \nabla h(\mathbf{W}^{(t)})\rangle + \frac{L}{2}\|\mathbf{B} - \mathbf{W}^{(t)}\|_{\ell_2}^2 + \lambda_1\|\boldsymbol{\omega}^\top\mathbf{B}_1\|_{\ell_1} + \lambda_2\|\boldsymbol{\omega}^\top\mathbf{B}_2\|_{\ell_1}\right\}\\ &\equiv \arg\min_{\mathbf{B}}\ L\left\{\frac{1}{2}\|\mathbf{B} - (\mathbf{W}^{(t)} - \frac{1}{L}\nabla h(\mathbf{W}^{(t)})\|_{\ell_2}^2 + \frac{\lambda_1}{L}\sum_{j=1}^{p_1}\sum_{k=1}^{m}\omega_k|\beta_{jk}| + \frac{\lambda_2}{L}\sum_{j=p_1+1}^{p_1+p_2}\sum_{k=1}^{m}\omega_k|\beta_{jk}|\right\}.\end{aligned}$$

Since $\mathbf{0}$ contains in its subgradient, that is

$$\begin{aligned}\mathbf{0} &= \partial\left(\frac{1}{2}\|\mathbf{B} - (\mathbf{W}^{(t)} - \frac{1}{L}\nabla h(\mathbf{W}^{(t)}))\|_{\ell_2}^2 + \frac{\lambda_1}{L}\sum_{j=1}^{p_1}\sum_{k=1}^{m}\omega_k|\beta_{jk}| + \frac{\lambda_2}{L}\sum_{j=p_1+1}^{p_1+p_2}\sum_{k=1}^{m}\omega_k|\beta_{jk}|\right)\\ &= \begin{bmatrix}\beta_0^\top - (\omega_0^{\top(t)} - \frac{1}{L}\nabla h(\omega_0^{\top(t)}))\\ \mathbf{B}_1 - (\mathbf{W}_1^{(t)} - \frac{1}{L}\nabla h(\mathbf{W}_1^{(t)})) + \partial\left(\frac{\lambda_1}{L}\sum_{j=1}^{p_1}\sum_{k=1}^{m}\omega_k|\beta_{jk}|\right)\\ \mathbf{B}_2 - (\mathbf{W}_2^{(t)} - \frac{1}{L}\nabla h(\mathbf{W}_2^{(t)})) + \partial\left(\frac{\lambda_2}{L}\sum_{j=p_1+1}^{p_1+p_2}\sum_{k=1}^{m}\omega_k|\beta_{jk}|\right)\end{bmatrix}.\end{aligned}$$

Thus, the closed-form solution for $\mathbf{B}^{(t+1)}$ is

$$\begin{aligned}
\beta_0^\top &= \omega_0^{\top(t)} - \frac{1}{L}\nabla h(\omega_0^{\top(t)}),\\
\beta_{jk} &= \operatorname{sign}(w_{jk}) \max\left(0, |w_{jk}| - \frac{\lambda_1 \omega_{\nu(k)}}{L}\right), j = 1, \cdots, p_1,\\
\beta_{jk} &= \operatorname{sign}(w_{jk}) \max\left(0, |w_{jk}| - \frac{\lambda_2 \omega_{\nu(k)}}{L}\right), j = p_1+1, \cdots, p_1+p_2,
\end{aligned}$$

where $w_{jk}$'s ($j = 1, \cdots, p_1$) are the elements of $\mathbf{W}_1^{(t)} - \frac{1}{L}\nabla h(\mathbf{W}_1^{(t)})$, $w_{jk}$'s ($j = p_1 + 1, \cdots, p_1 + p_2$) are the elements of $\mathbf{W}_2^{(t)} - \frac{1}{L}\nabla h(\mathbf{W}_2^{(t)})$, and $\omega_{\nu(k)}$ is the weight for the leaf node associated with the $k$th drug.

**S3.2 Directly adapted IPF-tree-lasso with non-penalized features**

The algorithm can also be applied not to shrink some specific features. Then the objective function of IPF-tree-lasso with two data sources is

$$\begin{aligned}
\min_{\boldsymbol{\beta}_0, \mathbf{B}} \{ &\frac{1}{2}\|\mathbf{Y} - \mathbf{1}\beta_0^\top - \mathbf{X}_0\mathbf{B}_0 - \mathbf{X}_1\mathbf{B}_1 - \mathbf{X}_2\mathbf{B}_2\|_F^2 + f_\mu(\mathbf{B}_1) + f_\mu(\mathbf{B}_2)\\
&+ \lambda_1 \sum_{j=1}^{p_1}\sum_{k=1}^{m} \omega_k |\beta_{jk}| + \lambda_2 \sum_{j=p_1+1}^{p_1+p_2}\sum_{k=1}^{m} \omega_k |\beta_{jk}| \},
\end{aligned}$$

where $\mathbf{B}_0$ is the coefficients matrix of non-penalized features $\mathbf{X}_0$, and $\mathbf{B} = [\beta_0 \vdots \mathbf{B}_0 \vdots \mathbf{B}_1 \vdots \mathbf{B}_2]$ The smooth part is

$$h(\mathbf{B}) = \frac{1}{2}\|\mathbf{Y} - \mathbf{1}\beta_0^\top - \mathbf{X}_0\mathbf{B}_0 - \mathbf{X}_1\mathbf{B}_1 - \mathbf{X}_2\mathbf{B}_2\|_F^2 + f_\mu(\mathbf{B}_1) + f_\mu(\mathbf{B}_2)$$

and its gradient is

$$\nabla h(\mathbf{B}) = \begin{bmatrix} \nabla h(\beta_0^\top) \\ \nabla h(\mathbf{B}_0) \\ \nabla h(\mathbf{B}_1) \\ \nabla h(\mathbf{B}_2) \end{bmatrix} = \mathbf{X}^\top\mathbf{X} \begin{bmatrix} \beta_0^\top \\ \mathbf{B}_0 \\ \mathbf{B}_1 \\ \mathbf{B}_2 \end{bmatrix} - \mathbf{X}^\top\mathbf{Y} + \begin{bmatrix} 0 & 0 & 0 & 0 \\ 0 & 0 & 0 & 0 \\ 0 & 0 & (\mathbf{A}_1^*)^\top & 0 \\ 0 & 0 & 0 & (\mathbf{A}_2^*)^\top \end{bmatrix} \begin{bmatrix} 0 \\ 0 \\ \lambda_1 \mathbb{I}_{p_1} \\ \lambda_2 \mathbb{I}_{p_2} \end{bmatrix} C,$$

with Lipschitz constant

$$L = \lambda_{\max}(\mathbf{X}^\top\mathbf{X}) + \frac{1}{\mu} \left\| \begin{bmatrix} 0 \\ 0 \\ \lambda_1 \mathbb{I}_{p_1} \\ \lambda_2 \mathbb{I}_{p_2} \end{bmatrix} C \right\|^2 .$$

By the subgradient,

$$\mathbf{0} = \partial\left(\frac{1}{2}\|\mathbf{B} - (\mathbf{W}^{(t)} - \frac{1}{L}\nabla h(\mathbf{W}^{(t)}))\|_{\ell_2}^2 + \frac{\lambda_1}{L}\sum_{j=1}^{p_1}\sum_{k=1}^{m}\omega_k|\beta_{jk}| + \frac{\lambda_2}{L}\sum_{j=p_1+1}^{p_1+p_2}\sum_{k=1}^{m}\omega_k|\beta_{jk}|\right)$$

$$= \begin{bmatrix} \beta_0^\top - (\omega_0^{\top(t)} - \frac{1}{L}\nabla h(\omega_0^{\top(t)})) \\ \mathbf{B}_0^\top - (\mathbf{W}_0^{(t)} - \frac{1}{L}\nabla h(\mathbf{W}_0^{(t)})) \\ \mathbf{B}_1 - (\mathbf{W}_1^{(t)} - \frac{1}{L}\nabla h(\mathbf{W}_1^{(t)}))\|_{\ell_2}^2 + \partial\left(\frac{\lambda_1}{L}\sum_{j=1}^{p_1}\sum_{k=1}^{m}\omega_k|\beta_{jk}|\right) \\ \mathbf{B}_2 - (\mathbf{W}_2^{(t)} - \frac{1}{L}\nabla h(\mathbf{W}_2^{(t)}))\|_{\ell_2}^2 + \partial\left(\frac{\lambda_2}{L}\sum_{j=p_1+1}^{p_1+p_2}\sum_{k=1}^{m}\omega_k|\beta_{jk}|\right) \end{bmatrix}.$$

Thus, the closed-form solution for $\mathbf{B}^{(t+1)}$ is

$$\begin{aligned} \beta_0^\top &= \omega_0^{\top(t)} - \frac{1}{L}\nabla h(\omega_0^{\top(t)}), \\ \mathbf{B}_0^\top &= \mathbf{W}_0^{(t)} - \frac{1}{L}\nabla h(\mathbf{W}_0^{(t)}), \\ \beta_{jk} &= \operatorname{sign}(w_{jk})\max\left(0, |w_{jk}| - \frac{\lambda_1\omega_{\nu(k)}}{L}\right), \\ \beta_{jk} &= \operatorname{sign}(w_{jk})\max\left(0, |w_{jk}| - \frac{\lambda_2\omega_{\nu(k)}}{L}\right). \end{aligned}$$

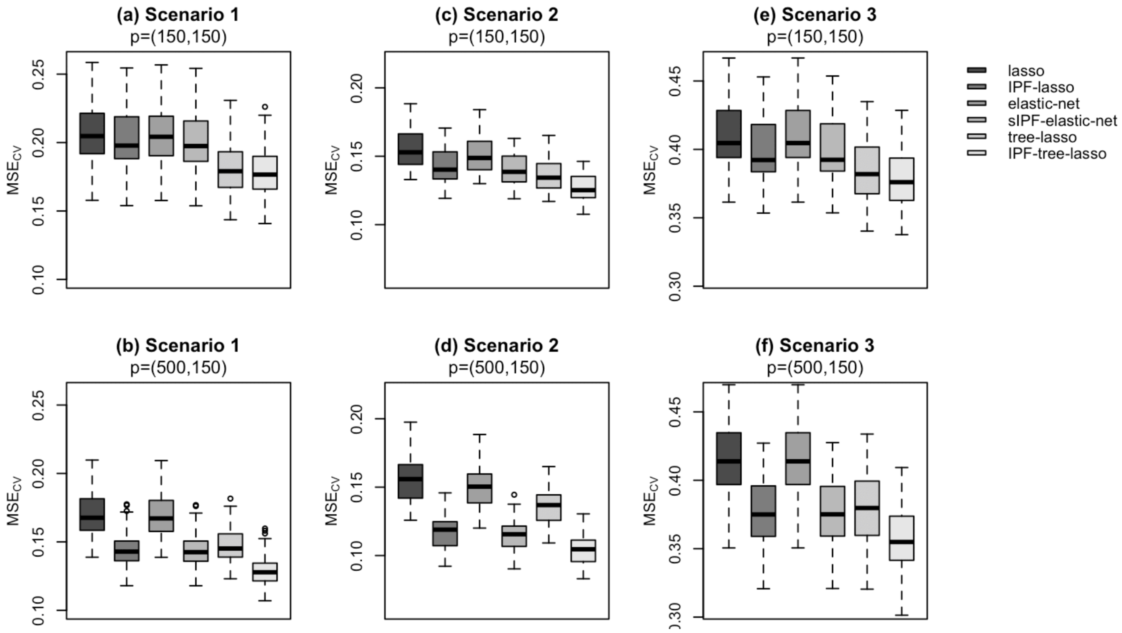


Fig. S4: Comparison of $\text{MSE}_{\text{CV}}$ between different structures of $\mathbf{Y}$ and different feature numbers of the two data sources. The first half boxes in each panel are based on the same feature number of $\mathbf{X}_1$ and $\mathbf{X}_2$, $p_1 = p_2 = 150$. The second half boxes in each panel are based on $p_1 = 500$ features of $\mathbf{X}_1$ and $p_2 = 150$ features of $\mathbf{X}_2$.

**S4. Comparison of MSE from cross-validation in simulation studies.** In the 50 simulations, the comparison of MSE from 5-fold cross-validation by all methods are shown in Figure S4.

**S5. Algorithm for the simulation study.** The Algorithm 1 below shows the procedure of the simulation study.

**Algorithm 1:** Simulation study setup to compare the prediction performance of penalized regression

**Input :** $\mathbf{X}$, $\mathbf{Y}$ and validation data $\mathbf{X}_{\text{val}}$, $\mathbf{Y}_{\text{val}}$ simulated according to simulation scenario 1, 2 or 3 with $(p_1, p_2) = (150, 150)$ or $(p_1, p_2) = (500, 150)$.

**Output:** Prediction performance of the 6 methods, i.e., lasso, elastic net, IPF-lasso, sIPF-elastic-net, tree-lasso, IPF-tree-lasso.

Use hierarchical clustering to obtain a tree $T$ representing the grouping structure in $\mathbf{Y}$.

Split data $\mathbf{X}$ and $\mathbf{Y}$ into $K = 5$ folds, respectively. $\mathbf{X}_{(-k)}$ and $\mathbf{Y}_{(-k)}$ exclude the observations of $k$th fold, and $\mathbf{X}_{(k)}$ and $\mathbf{Y}_{(k)}$ consist of the observations of $k$th fold.

**for** *method* $M = 1, \cdots, 6$ **do**

  **for** *penalty parameters* $\boldsymbol{\theta}_{M,l}(l = 1, \cdots, L_M)$ **do**

    **for** *fold* $k = 1, \cdots, K$ **do**

      i) Estimate $(\hat{\boldsymbol{\beta}}^M_{0(-k)}, \hat{\mathbf{B}}^M_{(-k)}) \leftarrow \underset{\boldsymbol{\beta}_0,\mathbf{B}}{\arg\min}\{\frac{1}{2mn}\|\mathbf{Y}_{(-k)} - \mathbf{1}_n\boldsymbol{\beta}_0^\top - \mathbf{X}_{(-k)}\mathbf{B}\|_F^2 + \text{pen}_M(\mathbf{B})\}$ by the $M$th method as outlined in Section 2.

      ii) Compute $\hat{\text{err}}^M_k(\boldsymbol{\theta}_{M,l}) \leftarrow \|\mathbf{Y}_{(k)} - \mathbf{1}_n\hat{\boldsymbol{\beta}}^{M\top}_{0(-k)} - \mathbf{X}_{(k)}\hat{\mathbf{B}}^M_{(-k)}\|_F^2$.

    **end**

    Compute cross-validation error $\text{MSE}^M_{\text{CV}}(\boldsymbol{\theta}_{M,l}) \leftarrow \frac{1}{K}\sum_{k=1}^K \hat{\text{err}}^M_k(\boldsymbol{\theta}_{M,l})$.

  **end**

  i) Obtain optimal penalty parameters $\boldsymbol{\theta}^{\text{opt}}_M \leftarrow \text{argmin}_{\boldsymbol{\theta}_{M,l}}\text{MSE}^M_{\text{CV}}(\boldsymbol{\theta}_{M,l})$.

  ii) Obtain $\hat{\boldsymbol{\beta}}^M_0$ and $\hat{\mathbf{B}}^M$ by fitting $M$th model on the full $\mathbf{X}$ and $\mathbf{Y}$ using$\boldsymbol{\theta}^{\text{opt}}_M$ .

  iii) Compute the final prediction error $\text{MSE}^M_{\text{val}}(\boldsymbol{\theta}^{\text{opt}}_M) \leftarrow \frac{1}{mn}\|\mathbf{Y}_{\text{val}} - \mathbf{1}_n\hat{\boldsymbol{\beta}}^{M\top}_0 - \mathbf{X}_{\text{val}}\hat{\mathbf{B}}^M\|_F^2$.

**end**

**Result:** $\text{MSE}^M_{\text{val}}$, $\hat{\boldsymbol{\beta}}^M_0$ and $\hat{\mathbf{B}}^M$ of all methods, $M = 1, \cdots, 6$.

**S6. Tree-lasso with non-penalized features.** After applying the Proposition 3 to transform IPF-tree-lasso to its equivalent tree-lasso problem, we can use original tree-lasso algorithm directly even including non-penalized features. Then the objective function of tree-lasso is

$$\min_{\boldsymbol{\beta}_0,\mathbf{B}}\left\{\frac{1}{2}\|\mathbf{Y} - \mathbf{1}\beta_0^\top - \mathbf{X}_0\mathbf{B}_0 - \mathbf{X}_1\mathbf{B}_1\|_F^2 + f_\mu(\mathbf{B}_1) + \lambda\sum_{j=1}^p\sum_{k=1}^m \omega_k|\beta_{jk}|\right\}.$$

The smooth part is

$$h(\mathbf{B}) = \|\mathbf{Y} - \mathbf{1}\beta_0^\top - \mathbf{X}_0\mathbf{B}_0 - \mathbf{X}_1\mathbf{B}_1\|_F^2 + f_\mu(\mathbf{B}_1)$$

and its gradient is

$$\nabla h(\mathbf{B}) = \begin{bmatrix} \nabla h(\beta_0^\top) \\ \nabla h(\mathbf{B}_0) \\ \nabla h(\mathbf{B}_1) \end{bmatrix} = \mathbf{X}^\top\mathbf{X} \begin{bmatrix} \beta_0^\top \\ \mathbf{B}_0 \\ \mathbf{B}_1 \end{bmatrix} - \mathbf{X}^\top\mathbf{Y} + \begin{bmatrix} 0 & 0 & 0 \\ 0 & 0 & 0 \\ 0 & 0 & (\mathbf{A}^*)^\top \end{bmatrix} \begin{bmatrix} 0 \\ 0 \\ \lambda\mathbb{I}_p \end{bmatrix} C,$$

with Lipschitz constant

$$L = \lambda_{\max}(\mathbf{X}^\top\mathbf{X}) + \frac{1}{\mu} \left\| \begin{bmatrix} 0 \\ 0 \\ \lambda\mathbb{I}_p \end{bmatrix} C \right\|^2.$$

By the subgradient,

$$\begin{aligned} \mathbf{0} &= \partial \left( \frac{1}{2} \|\mathbf{B} - (\mathbf{W}^{(t)} - \frac{1}{L}\nabla h(\mathbf{W}^{(t)}))\|_{\ell_2}^2 + \frac{\lambda}{L} \sum_{j=1}^{p} \sum_{k=1}^{m} \omega_k |\beta_{jk}| \right) \\ &= \begin{bmatrix} \beta_0^\top - (\omega_0^{\top(t)} - \frac{1}{L}\nabla h(\omega_0^{\top(t)})) \\ \mathbf{B}_0 - (\mathbf{W}_0^{(t)} - \frac{1}{L}\nabla h(\mathbf{W}_0^{(t)})) \\ \mathbf{B}_1 - (\mathbf{W}_1^{(t)} - \frac{1}{L}\nabla h(\mathbf{W}_1^{(t)})) + \partial \left( \frac{\lambda}{L} \sum_{j=1}^{p} \sum_{k=1}^{m} \omega_k |\beta_{jk}| \right) \end{bmatrix}. \end{aligned}$$

Thus, the closed-form solution for $\mathbf{B}^{(t+1)}$ is

$$\begin{aligned} \beta_0^\top &= \omega_0^{\top(t)} - \frac{1}{L}\nabla h(\omega_0^{\top(t)}), \\ \mathbf{B}_0 &= \mathbf{W}_0^{(t)} - \frac{1}{L}\nabla h(\mathbf{W}_0^{(t)}), \\ \beta_{jk} &= \text{sign}(w_j^k) \max \left( 0, |w_j^k| - \frac{\lambda \omega_{\nu(k)}}{L} \right). \end{aligned}$$

**S7. Additional results for individual drugs and tissues of the GDSC data analysis.**

Table S7.1 *Prediction $R^2$ for each method with respect to each drug in the GDSC data analysis*

| **Drug** | | Nutlin-3a | RDEA119 | Methotrexate | 17-AAG | PD-0325901 | CI-1040 | AZD6244 | Nilotinib | Bicalutamide | LFM-A13 | SL-0101-1 | CCT007093 | NSC-87877 | ABT-888 |
|---|---|---|---|---|---|---|---|---|---|---|---|---|---|---|---|
| **Tissue** | *N* | | | | | | | | NULL | | | | | | |
| digestive system | 50 | -0.006 | 0.017 | 0.029 | 0.010 | 0.048 | 0.022 | -0.028 | -0.008 | -0.136 | 0.035 | -0.064 | -0.005 | -0.014 | 0.030 |
| urogenital system | 43 | 0.007 | -0.044 | -0.030 | -0.013 | -0.084 | -0.016 | -0.073 | -0.062 | -0.023 | -0.019 | -0.037 | 0.005 | -0.006 | -0.041 |
| blood | 77 | -0.010 | -0.039 | -0.010 | 0.015 | -0.076 | -0.034 | 0.023 | -0.001 | 0.069 | -0.032 | -0.015 | -0.003 | -0.018 | -0.033 |
| kidney | 14 | 0.017 | -0.053 | 0.011 | -0.052 | -0.097 | -0.022 | -0.106 | -0.048 | 0.021 | -0.168 | -0.041 | -0.017 | -0.006 | -0.057 |
| nervous system | 60 | -0.009 | 0.002 | 0.005 | -0.035 | 0.005 | -0.021 | -0.010 | 0.022 | 0.001 | -0.039 | -0.001 | -0.018 | -0.064 | 0.014 |
| thyroid | 9 | -0.045 | -0.077 | -0.084 | -0.150 | 0.063 | -0.062 | -0.009 | -0.053 | -0.212 | -0.257 | -0.001 | -0.020 | -0.007 | -0.097 |
| skin | 32 | 0.018 | -0.010 | -0.005 | -0.015 | 0.020 | 0.003 | -0.049 | -0.012 | -0.027 | 0.046 | -0.005 | -0.001 | 0.008 | -0.014 |
| soft tissue | 13 | -0.046 | 0.004 | 0.012 | -0.013 | -0.117 | 0.011 | 0.032 | -0.104 | 0.117 | 0.040 | 0.001 | -0.002 | -0.029 | 0.015 |
| aerodigestive tract | 43 | -0.029 | -0.020 | -0.002 | -0.042 | -0.012 | 0.045 | -0.054 | -0.002 | -0.086 | -0.048 | -0.004 | -0.014 | 0.021 | 0.042 |
| lung | 89 | -0.017 | -0.005 | -0.008 | -0.005 | -0.031 | -0.008 | 0.040 | 0.027 | 0.025 | 0.002 | -0.013 | -0.007 | -0.031 | 0.011 |
| pancreas | 14 | -0.038 | 0.008 | -0.011 | -0.035 | -0.023 | -0.007 | -0.038 | -0.126 | 0.029 | 0.018 | 0.052 | -0.001 | 0.083 | 0.099 |
| breast | 29 | -0.035 | -0.101 | 0.026 | 0.001 | -0.107 | -0.087 | -0.028 | -0.058 | -0.114 | -0.042 | 0.016 | -0.030 | -0.010 | 0.045 |
| bone | 25 | 0.017 | 0.026 | -0.033 | 0.015 | 0.040 | 0.000 | 0.023 | 0.003 | -0.117 | -0.005 | 0.051 | -0.003 | 0.010 | -0.050 |
| **Tissue** | | | | | | | | | OLS | | | | | | |
| digestive system | | -0.034 | 0.215 | 0.019 | -0.012 | 0.155 | 0.222 | 0.108 | 0.112 | -0.165 | 0.094 | -0.116 | -0.056 | 0.021 | 0.062 |
| urogenital system | | -0.017 | -0.090 | -0.064 | 0.113 | -0.130 | -0.054 | -0.196 | 0.060 | 0.036 | -0.008 | -0.062 | -0.029 | -0.019 | -0.075 |
| blood | | 0.011 | 0.187 | 0.709 | 0.457 | 0.220 | 0.022 | 0.275 | -0.040 | 0.355 | -0.091 | -0.008 | 0.007 | 0.165 | -0.114 |
| kidney | | 0.067 | -0.337 | 0.387 | 0.205 | -0.203 | -0.157 | -0.169 | -0.458 | -0.108 | -16.179 | -1.766 | -0.160 | -0.012 | -0.538 |
| nervous system | | -0.086 | -0.012 | 0.300 | -0.062 | -0.036 | -0.046 | -0.014 | 0.134 | -0.026 | -0.098 | -0.016 | -0.113 | -0.062 | -0.015 |
| thyroid | | -0.056 | -1.145 | -0.161 | 0.053 | -1.149 | -1.507 | 0.210 | -2.530 | -0.700 | -0.972 | -1.290 | -0.924 | -0.549 | -0.874 |
| skin | | 0.052 | 0.353 | 0.132 | 0.502 | 0.523 | 0.228 | -0.029 | -0.040 | -0.136 | -0.013 | -0.064 | -0.018 | -0.152 | -0.035 |
| soft tissue | | -0.370 | 0.112 | 0.285 | -0.120 | -0.530 | -0.053 | -0.236 | -0.376 | -0.147 | -1.631 | -1.762 | -0.222 | -0.603 | 0.090 |
| aerodigestive tract | | 0.292 | 0.037 | -0.003 | 0.069 | -0.150 | -0.083 | -0.078 | 0.184 | -0.208 | -0.092 | -0.044 | -0.081 | -0.209 | -0.059 |
| lung | | 0.044 | 0.142 | -0.019 | -0.016 | 0.147 | 0.093 | 0.108 | 0.039 | 0.014 | -0.003 | -0.025 | -0.011 | -0.018 | 0.008 |
| pancreas | | 0.791 | 0.277 | 0.607 | 0.616 | 0.446 | 0.468 | -0.376 | 0.441 | -0.156 | 0.392 | -0.078 | -0.080 | -0.080 | -0.200 |
| breast | | -0.057 | -0.022 | 0.551 | -0.012 | 0.007 | 0.071 | 0.140 | -0.033 | -0.257 | -0.160 | -0.071 | -0.374 | -0.205 | 0.192 |
| bone | | -0.084 | -0.065 | -0.346 | -0.243 | -0.254 | -0.553 | -0.002 | -0.136 | -0.098 | 0.260 | 0.270 | -0.085 | -0.400 | -0.279 |
| **Tissue** | | | | | | | | | Lasso | | | | | | |
| digestive system | | 0.281 | 0.246 | 0.019 | 0.016 | 0.147 | 0.199 | 0.112 | 0.112 | -0.165 | 0.094 | -0.116 | -0.056 | 0.021 | 0.062 |
| urogenital system | | 0.182 | -0.006 | -0.067 | 0.102 | -0.036 | -0.045 | -0.191 | 0.058 | 0.036 | -0.008 | -0.062 | -0.029 | -0.019 | -0.075 |
| blood | | 0.276 | 0.369 | 0.709 | 0.469 | 0.352 | 0.075 | 0.281 | 0.330 | 0.355 | -0.091 | -0.008 | 0.007 | 0.165 | -0.114 |
| kidney | | 0.466 | -0.395 | 0.409 | 0.171 | -0.238 | -0.157 | -0.077 | -0.458 | -0.108 | -16.179 | -1.766 | -0.160 | -0.012 | -0.538 |
| nervous system | | 0.297 | 0.010 | 0.296 | 0.164 | -0.045 | -0.071 | -0.040 | 0.134 | -0.026 | -0.098 | -0.016 | -0.113 | -0.062 | -0.015 |
| thyroid | | 0.206 | -0.788 | -0.157 | 0.232 | -0.804 | -1.011 | 0.214 | -2.511 | -0.700 | -0.972 | -1.290 | -0.924 | -0.549 | -0.874 |
| skin | | 0.366 | 0.304 | 0.132 | 0.518 | 0.493 | 0.194 | -0.039 | -0.040 | -0.136 | -0.013 | -0.064 | -0.018 | -0.152 | -0.035 |
| soft tissue | | 0.211 | 0.371 | 0.340 | -0.073 | -0.537 | 0.024 | -0.244 | -0.376 | -0.147 | -1.631 | -1.762 | -0.222 | -0.603 | 0.090 |
| aerodigestive tract | | 0.402 | -0.038 | -0.002 | 0.064 | -0.140 | -0.049 | -0.076 | 0.184 | -0.208 | -0.092 | -0.044 | -0.081 | -0.209 | -0.059 |
| lung | | 0.282 | 0.336 | -0.011 | 0.062 | 0.223 | 0.174 | 0.121 | 0.039 | 0.014 | -0.003 | -0.025 | -0.011 | -0.018 | 0.008 |
| pancreas | | 0.884 | 0.220 | 0.608 | 0.586 | 0.425 | 0.458 | -0.387 | 0.442 | -0.156 | 0.392 | -0.078 | -0.080 | -0.080 | -0.200 |
| breast | | -0.007 | 0.051 | 0.549 | -0.050 | 0.033 | 0.120 | 0.141 | -0.034 | -0.257 | -0.160 | -0.071 | -0.374 | -0.205 | 0.192 |
| bone | | 0.275 | 0.135 | -0.340 | -0.155 | -0.149 | -0.519 | -0.003 | -0.137 | -0.098 | 0.260 | 0.270 | -0.085 | -0.400 | -0.279 |
| **Tissue** | | | | | | | | | IPF-lasso | | | | | | |
| digestive system | | 0.286 | 0.270 | 0.033 | 0.061 | 0.182 | 0.181 | 0.115 | 0.110 | -0.165 | 0.094 | -0.116 | -0.056 | 0.021 | 0.062 |
| urogenital system | | 0.166 | 0.078 | -0.076 | 0.099 | 0.013 | -0.010 | -0.180 | 0.054 | 0.036 | -0.008 | -0.062 | -0.029 | -0.019 | -0.075 |
| blood | | 0.259 | 0.419 | 0.707 | 0.483 | 0.403 | 0.149 | 0.268 | 0.323 | 0.355 | -0.091 | -0.008 | 0.007 | 0.165 | -0.114 |
| kidney | | 0.437 | -0.264 | 0.406 | 0.230 | -0.223 | -0.109 | -0.061 | -0.443 | -0.108 | -16.179 | -1.766 | -0.160 | -0.012 | -0.538 |
| nervous system | | 0.295 | 0.051 | 0.294 | 0.218 | 0.008 | -0.059 | -0.061 | 0.133 | -0.026 | -0.098 | -0.016 | -0.113 | -0.062 | -0.015 |
| thyroid | | 0.230 | -0.562 | -0.173 | 0.266 | -0.523 | -0.664 | 0.277 | -2.512 | -0.700 | -0.972 | -1.290 | -0.924 | -0.549 | -0.874 |
| skin | | 0.359 | 0.286 | 0.140 | 0.518 | 0.477 | 0.165 | -0.042 | -0.038 | -0.136 | -0.013 | -0.064 | -0.018 | -0.152 | -0.035 |
| soft tissue | | 0.232 | 0.486 | 0.452 | -0.065 | -0.486 | 0.100 | -0.183 | -0.385 | -0.147 | -1.631 | -1.762 | -0.222 | -0.603 | 0.090 |
| aerodigestive tract | | 0.382 | -0.035 | -0.011 | 0.084 | -0.115 | -0.015 | -0.047 | 0.184 | -0.208 | -0.092 | -0.044 | -0.081 | -0.209 | -0.059 |
| lung | | 0.292 | 0.373 | -0.007 | 0.073 | 0.271 | 0.243 | 0.165 | 0.041 | 0.014 | -0.003 | -0.025 | -0.011 | -0.018 | 0.008 |
| pancreas | | 0.868 | 0.163 | 0.603 | 0.589 | 0.375 | 0.448 | -0.403 | 0.441 | -0.156 | 0.392 | -0.078 | -0.080 | -0.080 | -0.200 |
| breast | | -0.033 | 0.052 | 0.546 | -0.081 | 0.009 | 0.129 | 0.144 | -0.034 | -0.257 | -0.160 | -0.071 | -0.374 | -0.205 | 0.192 |
| bone | | 0.287 | 0.152 | -0.277 | -0.030 | -0.092 | -0.457 | -0.008 | -0.141 | -0.098 | 0.260 | 0.270 | -0.085 | -0.400 | -0.279 |
| **Tissue** | | | | | | | | | Elastic net | | | | | | |
| digestive system | | 0.282 | 0.245 | 0.020 | 0.020 | 0.148 | 0.198 | 0.113 | 0.112 | -0.165 | 0.094 | -0.116 | -0.056 | 0.021 | 0.062 |
| urogenital system | | 0.192 | -0.002 | -0.068 | 0.101 | -0.033 | -0.039 | -0.191 | 0.059 | 0.036 | -0.008 | -0.062 | -0.029 | -0.019 | -0.075 |
| blood | | 0.273 | 0.377 | 0.709 | 0.469 | 0.362 | 0.084 | 0.280 | 0.328 | 0.355 | -0.091 | -0.008 | 0.007 | 0.165 | -0.114 |
| kidney | | 0.486 | -0.354 | 0.409 | 0.172 | -0.242 | -0.134 | -0.087 | -0.458 | -0.108 | -16.179 | -1.766 | -0.160 | -0.012 | -0.538 |
| nervous system | | 0.290 | 0.019 | 0.296 | 0.175 | -0.032 | -0.067 | -0.039 | 0.134 | -0.026 | -0.098 | -0.016 | -0.113 | -0.062 | -0.015 |
| thyroid | | 0.188 | -0.767 | -0.158 | 0.235 | -0.811 | -1.039 | 0.214 | -2.512 | -0.700 | -0.972 | -1.290 | -0.924 | -0.549 | -0.874 |
| skin | | 0.361 | 0.302 | 0.133 | 0.514 | 0.493 | 0.194 | -0.039 | -0.040 | -0.136 | -0.013 | -0.064 | -0.018 | -0.152 | -0.035 |
| soft tissue | | 0.210 | 0.386 | 0.339 | -0.063 | -0.522 | 0.028 | -0.244 | -0.376 | -0.147 | -1.631 | -1.762 | -0.222 | -0.603 | 0.090 |
| aerodigestive tract | | 0.393 | -0.032 | -0.001 | 0.064 | -0.136 | -0.050 | -0.075 | 0.184 | -0.208 | -0.092 | -0.044 | -0.081 | -0.209 | -0.059 |
| lung | | 0.284 | 0.337 | -0.012 | 0.065 | 0.226 | 0.179 | 0.121 | 0.039 | 0.014 | -0.003 | -0.025 | -0.011 | -0.018 | 0.008 |
| pancreas | | 0.881 | 0.216 | 0.609 | 0.588 | 0.417 | 0.455 | -0.386 | 0.442 | -0.156 | 0.392 | -0.078 | -0.080 | -0.080 | -0.200 |
| breast | | 0.010 | 0.046 | 0.550 | -0.045 | 0.028 | 0.117 | 0.142 | -0.034 | -0.257 | -0.160 | -0.071 | -0.374 | -0.205 | 0.192 |
| bone | | 0.257 | 0.138 | -0.340 | -0.142 | -0.156 | -0.520 | -0.003 | -0.137 | -0.098 | 0.260 | 0.270 | -0.085 | -0.400 | -0.279 |
| **Tissue** | | | | | | | | | sIPF-elastic-net | | | | | | |
| digestive system | | 0.184 | 0.291 | 0.040 | 0.063 | 0.198 | 0.216 | 0.129 | 0.114 | -0.169 | 0.078 | -0.107 | -0.051 | 0.015 | 0.067 |
| urogenital system | | 0.108 | 0.074 | -0.063 | 0.107 | -0.005 | -0.010 | -0.152 | 0.054 | 0.038 | -0.006 | -0.064 | -0.033 | -0.022 | -0.077 |
| blood | | 0.166 | 0.368 | 0.707 | 0.485 | 0.365 | 0.116 | 0.276 | 0.235 | 0.353 | -0.091 | -0.008 | 0.006 | 0.161 | -0.114 |
| kidney | | 0.371 | -0.352 | 0.420 | 0.254 | -0.181 | -0.070 | -0.021 | -0.468 | -0.088 | -16.174 | -1.680 | -0.156 | -0.011 | -0.548 |
| nervous system | | 0.168 | 0.037 | 0.295 | 0.192 | -0.030 | -0.037 | -0.030 | 0.136 | -0.024 | -0.095 | -0.019 | -0.115 | -0.059 | -0.015 |
| thyroid | | 0.136 | -0.751 | -0.153 | 0.242 | -0.824 | -0.840 | 0.301 | -2.477 | -0.742 | -0.927 | -1.339 | -0.925 | -0.532 | -0.831 |
| skin | | 0.274 | 0.300 | 0.140 | 0.526 | 0.480 | 0.179 | -0.045 | -0.036 | -0.140 | -0.010 | -0.066 | -0.022 | -0.153 | -0.030 |
| soft tissue | | -0.099 | 0.418 | 0.465 | -0.025 | -0.426 | 0.091 | -0.156 | -0.380 | -0.129 | -1.663 | -1.791 | -0.226 | -0.598 | 0.091 |
| aerodigestive tract | | 0.392 | 0.010 | -0.008 | 0.097 | -0.106 | -0.001 | -0.036 | 0.182 | -0.213 | -0.091 | -0.039 | -0.083 | -0.210 | -0.056 |
| lung | | 0.222 | 0.371 | 0.003 | 0.085 | 0.271 | 0.237 | 0.175 | 0.034 | 0.033 | 0.006 | -0.021 | -0.002 | -0.016 | 0.007 |
| pancreas | | 0.875 | 0.216 | 0.614 | 0.600 | 0.433 | 0.467 | -0.397 | 0.453 | -0.150 | 0.392 | -0.071 | -0.076 | -0.082 | -0.186 |
| breast | | -0.081 | 0.022 | 0.547 | -0.074 | 0.042 | 0.121 | 0.159 | -0.036 | -0.272 | -0.172 | -0.076 | -0.373 | -0.207 | 0.198 |
| bone | | 0.177 | 0.117 | -0.267 | -0.047 | -0.100 | -0.474 | -0.001 | -0.139 | -0.117 | 0.261 | 0.270 | -0.089 | -0.382 | -0.287 |
| **Tissue** | | | | | | | | | tree-lasso | | | | | | |
| digestive system | | 0.285 | 0.419 | 0.063 | 0.240 | 0.425 | 0.347 | 0.187 | -0.151 | -1.221 | -0.187 | -0.333 | -0.632 | -0.249 | -0.489 |
| urogenital system | | 0.061 | 0.169 | -0.121 | 0.329 | 0.158 | 0.119 | 0.066 | -0.582 | -0.456 | -0.165 | -0.123 | -0.594 | -0.518 | -0.210 |
| blood | | 0.409 | 0.520 | 0.643 | 0.571 | 0.502 | 0.256 | 0.289 | 0.014 | 0.275 | -0.136 | -0.109 | -0.131 | -0.329 | -0.440 |
| kidney | | 0.485 | -0.229 | 0.466 | 0.197 | -0.004 | 0.293 | 0.213 | -0.439 | -0.002 | -2.929 | -0.462 | -0.527 | -0.446 | -0.478 |
| nervous system | | 0.208 | 0.245 | 0.185 | 0.219 | 0.127 | 0.007 | 0.034 | -0.042 | -0.123 | -0.392 | -0.303 | -0.067 | -0.555 | -0.272 |
| thyroid | | 0.088 | 0.345 | -0.355 | 0.574 | 0.217 | 0.423 | -0.073 | 0.054 | -0.228 | -0.467 | -0.907 | -0.377 | 0.191 | -0.059 |
| skin | | 0.521 | 0.322 | 0.225 | 0.322 | 0.520 | 0.258 | -0.067 | -0.169 | -0.743 | -0.043 | -0.175 | -0.356 | -0.400 | 0.089 |
| soft tissue | | 0.506 | 0.661 | 0.260 | 0.527 | -0.132 | 0.260 | 0.238 | -0.444 | 0.008 | -0.398 | -1.523 | 0.001 | 0.090 | -0.297 |
| aerodigestive tract | | -0.151 | 0.283 | -0.042 | 0.279 | -0.007 | -0.231 | 0.069 | -0.012 | -0.366 | -0.340 | -0.278 | -0.197 | -0.387 | -0.010 |
| lung | | 0.435 | 0.445 | 0.060 | 0.182 | 0.308 | 0.423 | 0.342 | -0.081 | -0.093 | -0.039 | -0.158 | -0.077 | -0.154 | -0.024 |
| pancreas | | 0.386 | 0.437 | 0.336 | 0.665 | 0.602 | 0.606 | 0.047 | 0.691 | -2.669 | -0.044 | -0.197 | -0.564 | -0.875 | -2.095 |
| breast | | 0.023 | 0.178 | 0.533 | -0.336 | 0.143 | 0.187 | 0.045 | 0.015 | -0.350 | -0.454 | -0.688 | -0.555 | -0.409 | -0.639 |
| bone | | 0.451 | 0.423 | 0.183 | -0.048 | -0.067 | -0.106 | 0.278 | -0.239 | -3,092 | -0.386 | -0.677 | -0.643 | -0.938 | -0.252 |
| **Tissue** | | | | | | | | | IPF-tree-lasso | | | | | | |
| digestive system | | 0.380 | 0.407 | 0.030 | 0.233 | 0.444 | 0.349 | 0.223 | -0.021 | -1.181 | -0.096 | -0.365 | -0.595 | -0.157 | -0.399 |
| urogenital system | | 0.183 | 0.207 | -0.159 | 0.306 | 0.188 | 0.153 | 0.072 | -0.321 | -0.240 | -0.066 | -0.081 | -0.469 | -0.405 | -0.0840 |
| blood | | 0.422 | 0.526 | 0.659 | 0.575 | 0.492 | 0.233 | 0.277 | -0.069 | 0.234 | -0.256 | -0.116 | -0.171 | -0.334 | -0.557 |
| kidney | | 0.649 | -0.153 | 0.456 | 0.430 | -0.312 | 0.202 | 0.340 | -0.397 | -0.151 | -2.685 | -0.353 | -0.552 | -0.751 | -0.307 |
| nervous system | | 0.456 | 0.281 | 0.215 | 0.256 | 0.164 | 0.053 | 0.070 | -0.011 | -0.223 | -0.366 | -0.189 | -0.040 | -0.395 | -0.219 |
| thyroid | | 0.054 | 0.329 | -0.055 | 0.587 | 0.017 | 0.584 | 0.163 | -0.287 | -0.291 | -0.851 | -1.330 | -0.150 | 0.207 | -0.073 |
| skin | | 0.544 | 0.373 | 0.286 | 0.364 | 0.571 | 0.300 | -0.062 | -0.079 | -0.262 | -0.132 | -0.243 | -0.196 | -0.321 | 0.131 |
| soft tissue | | 0.696 | 0.648 | 0.445 | 0.571 | -0.163 | 0.267 | 0.261 | -0.072 | -0.128 | 0.140 | -1.038 | -0.008 | -0.020 | -0.127 |
| aerodigestive tract | | 0.216 | 0.234 | -0.021 | 0.223 | -0.041 | -0.224 | 0.181 | -0.010 | -0.410 | -0.332 | -0.223 | -0.094 | -0.312 | 0.044 |
| lung | | 0.417 | 0.429 | 0.131 | 0.205 | 0.298 | 0.372 | 0.341 | -0.035 | -0.100 | 0.001 | -0.127 | -0.119 | -0.093 | -0.084 |
| pancreas | | 0.663 | 0.373 | 0.418 | 0.635 | 0.600 | 0.553 | -0.123 | 0.423 | -2.857 | 0.124 | -0.359 | -0.400 | -0.804 | -3.077 |
| breast | | -0.015 | 0.143 | 0.526 | -0.249 | 0.153 | 0.202 | 0.194 | 0.055 | -0.427 | -0.520 | -0.433 | -0.345 | -0.291 | -0.347 |
| bone | | 0.556 | 0.382 | 0.182 | -0.037 | -0.084 | -0.125 | 0.251 | -0.136 | -2.613 | -0.264 | -0.147 | -0.309 | -0.619 | -0.244 |

All results are the average of 10 repetitions dividing training and external test data sets. The $N$ denotes the total number of cell lines of each cancer tissue type.

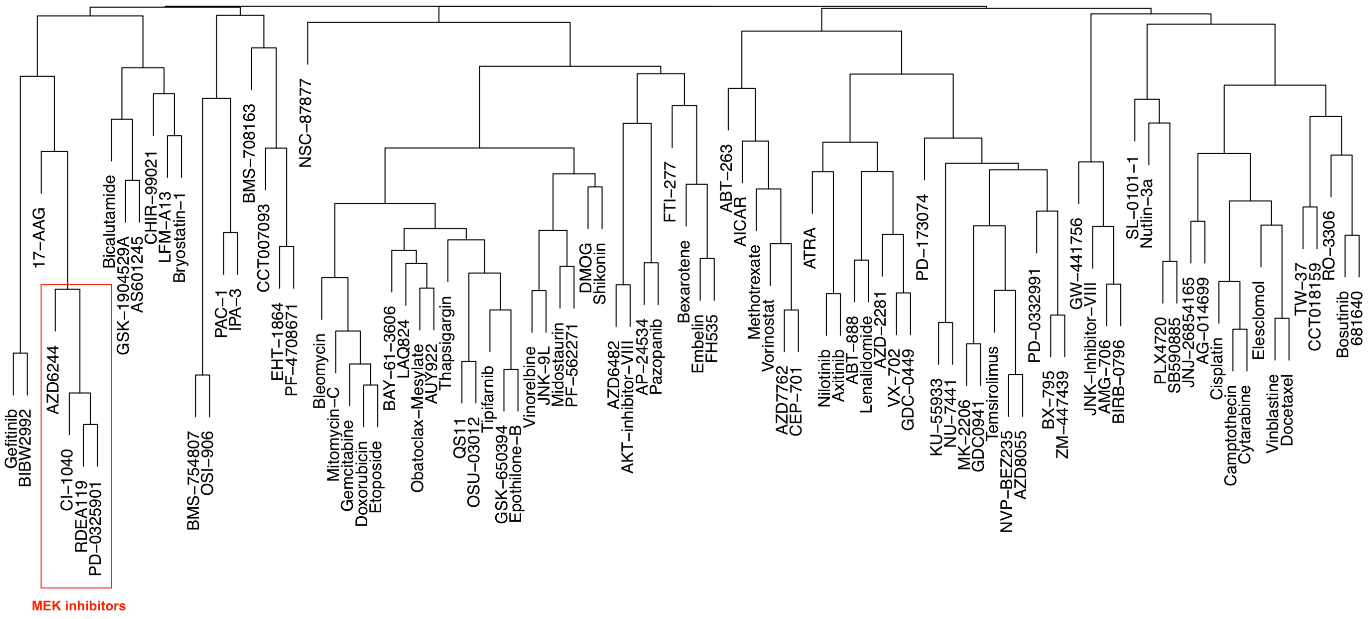


Fig S7.1: Dendrogram of the 97 drugs in the GDSC data.

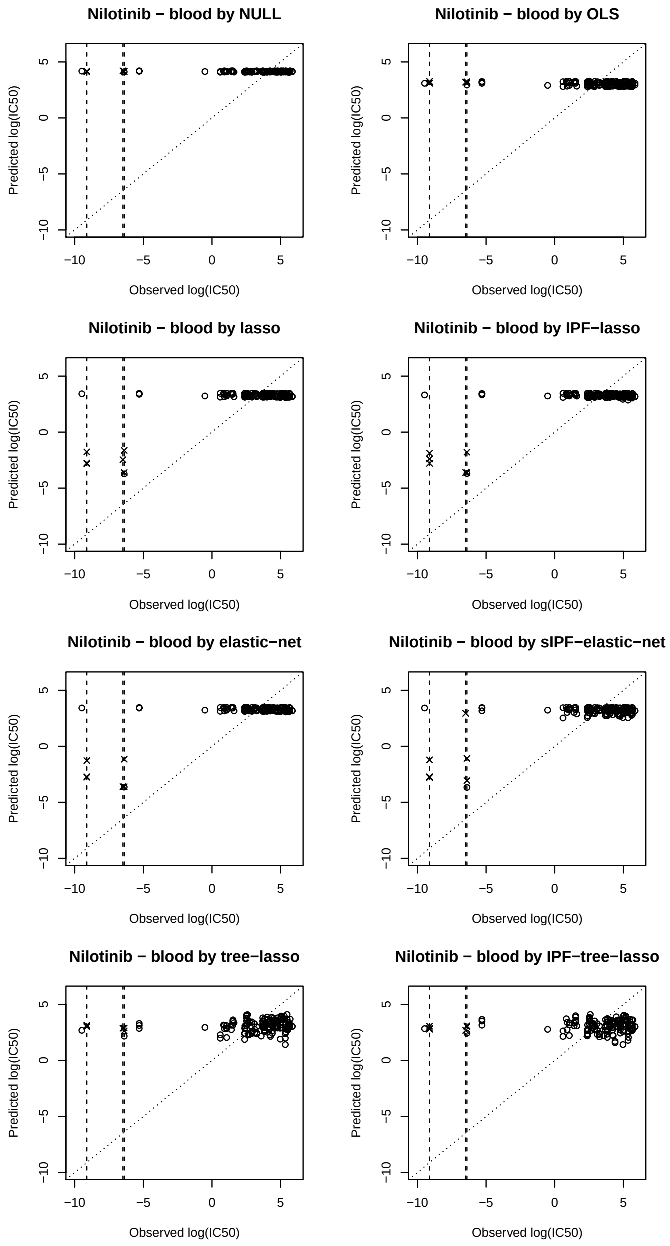


Fig S7.2: Prediction of blood cell lines treated by drug Nilotinib. Each point denotes the observed $\log(\mathrm{IC}_{50})$ vs. predicted $\log(\mathrm{IC}_{50})$ of one repetition. Points"$\times$" correspond to the BCR-ABL mutated blood cell lines. The three vertical dashed "----" lines in each plot indicate the three BCR-ABL mutated blood cell lines.

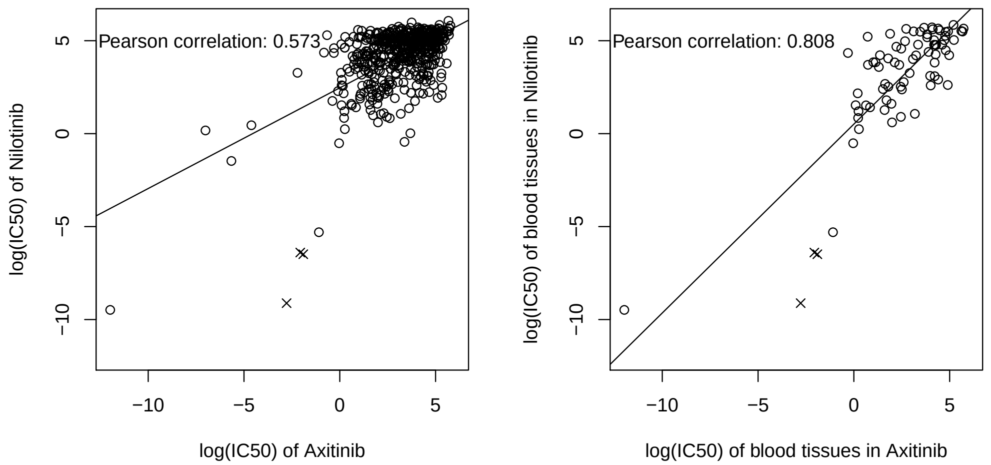


Fig S7.3: Scatter plots of $\log(\mathrm{IC}_{50})$ in drugs Nilotinib and Axitinib. The left panel shows the $\log(\mathrm{IC}_{50})$ of all cell lines in the two drugs and the right panel shows the $\log(\mathrm{IC}_{50})$ of the blood cell lines in the two drugs. Points"$\times$" correspond to the BCR-ABL mutated blood cell lines. The solid lines are linear regression lines.

Table S7.2 *Target genes selected by all methods (except sIPF-elastic-net, which selects all features) for corresponding drugs with $R^2_{val} > 0.100$. Gene names are mutation features with suffix ".MUT", copy number variation features with suffix ".CN" and gene expression features without suffix.*

| Drug | Target gene | Effector pathway/ biological process | Lasso | Elastic net | IPF-lasso | Tree-lasso | IPF-tree-lasso |
|---|---|---|---|---|---|---|---|
| **Nutlin-3$\alpha$** | MDM2 | MDM2-p53 interaction | TP53.MUT | | | TP53.MUT, TP53.CN | |
| **Nilotinib** | ABL | BCR-ABL fusion | BCR-ABL.MUT | | | - | BCR-ABL.MUT |
| **PLX4720** | B-Raf | Ras-Raf-MEK-ERK signalling* | B-Raf.MUT | | | RAF1.CN | B-Raf.MUT |
| **SB590885** | | | | | | | |
| **BIBW2992** | EGFR, ErbB2 | | ErbB2.MUT | | - | - | EGFR.MUT, ErbB2.MUT |
| **RDEA-119** | MEK1/2 | | B-Raf.MUT, NRAS.MUT | | B-Raf.MUT | RAF1.CN, NRAS.CN RASGRP1, RASGRP3 | B-Raf.MUT, KRAS.MUT NRAS.MUT, RASGRP3 |
| **PD-0325901** | | | NRAS.MUT | | | NRAS.CN, RASGRP1 | |
| **CI-1040** | | | - | | | RAF1.CN, NRAS.CN RASGRP1 | |
| **AZD6244** | | | B-Raf.MUT | | - | RASGRP1 | B-Raf.MUT, KRAS.MUT RASGRP1 RASGRP3 |

$*$ For the Ras-Raf-MEK-ERK signalling pathway we only consider the RAS, RAF, MEK and ERK gene families as target genes.

## REFERENCES

[1] Kim, S. and Xing, E.(2012). Tree-guide group lasso for multi-response regression with structured sparsity, with an application to eQTL mapping. *The Annals of Applied Statistics* **6**, 1095-1117.
